# Supplementary material for: Skew-Cyclic Codes over $B_k$
Source: arXiv:1705.06007 source file (2017-05-17)
Supplement: Supplementary file 1 [file Irwansyah-99-131-1-SM-2017.pdf]

## Codes over an infinite family of algebras

Research Article

Irwansyah\*, Intan Muchtadi-Alamsyah\*\*, Ahmad Muchlis, Aleams Barra\*\*, Djoko Suprijanto

**Abstract:** In this paper, we will show some properties of codes over the ring  $B_k = \mathbb{F}_p[v_1, \dots, v_k]/(v_i^2 = v_i, \forall i = 1, \dots, k)$ . These rings, form a family of commutative algebras over finite field  $\mathbb{F}_p$ . We first discuss about the form of maximal ideals and characterization of automorphisms for the ring  $B_k$ . Then, we define certain Gray map which can be used to give a connection between codes over  $B_k$  and codes over  $\mathbb{F}_p$ . Using the previous connection, we give a characterization for equivalence of codes over  $B_k$  and Euclidean self-dual codes. Furthermore, we give generators for invariant ring of Euclidean self-dual codes over  $B_k$  through MacWilliams relation of Hamming weight enumerator for such codes.

2010 MSC: 11T71

**Keywords:** Gray map, Equivalence of codes, Euclidean self-dual, Hamming weight enumerator, MacWilliams relation, Invariant ring

### 1. Introduction

Codes over finite rings has been an interesting topic in algebraic coding theory since the discovery of codes over  $\mathbb{Z}_4$ , see [4]. An example of finite rings which has interesting properties is the ring  $A_k = \mathbb{F}_2[v_1, \dots, v_k]$ , where  $v_i^2 = v_i$ , for  $1 \leq i \leq k$ , because it has two Gray maps which relate codes over such ring and binary codes, see [2]. This ring also has non-trivial automorphisms which can be used to define skew-cyclic codes, for example in [1], skew-cyclic codes over the ring  $A_1 = \mathbb{F}_2 + v\mathbb{F}_2$ , where  $v^2 = v$ , which give some optimal Euclidean and Hermitian self-dual codes. Furthermore, Abualrub *et al.* show that skew-cyclic codes over  $A_1$  have a connection to left submodules over a skew-polynomial ring and

\* The author is supported by Beasiswa Unggulan BPKLN Direktorat Jenderal Pendidikan Tinggi.

\*\* The authors are supported by Hibah Desentralisasi DIKTI 2016.

Irwansyah (Corresponding Author); Algebra Research Group, Institut Teknologi Bandung, Bandung, Indonesia, and Department of Mathematics, Universitas Mataram, Mataram, Indonesia (email: irw@unram.ac.id).

Intan Muchtadi-Alamsyah, Ahmad Muchlis, Aleams Barra; Algebra Research Group, Institut Teknologi Bandung, Bandung, Indonesia (email: ntan@math.itb.ac.id, muchlis@math.itb.ac.id, barra@math.itb.ac.id).

Djoko Suprijanto; Combinatorial Research Group, Institut Teknologi Bandung, Bandung, Indonesia (email: djoko@math.itb.ac.id).

give skew-polynomial generators for these codes. In [6], skew-cyclic codes over the ring  $A_1$  have been characterized using a Gray map. This characterization gives a way to construct skew-cyclic codes over the ring  $A_1$  from binary cyclic or quasi-cyclic codes, and also gives decoding algorithm for some codes over such ring. Meanwhile, Gao [3] consider skew-cyclic codes over the ring  $B_1 = \mathbb{F}_p + v\mathbb{F}_p$ , where  $v^2 = v$ , and found that these codes are equivalent to either cyclic codes or quasi-cyclic codes. Using this connection, Gao is able to give an enumeration for skew-cyclic codes which are constructed using an automorphism with order relatively prime to the length of the codes.

In this paper, we consider codes over the ring  $B_k = \mathbb{F}_p[v_1, \dots, v_k]$ , where  $v_i^2 = v_i$  for  $1 \leq i \leq k$ , which is a generalization of the ring  $A_k$  in [2] and  $B_1$  in [3]. We study its maximal ideals, automorphisms, equivalence codes, and Euclidean self-dual codes over these rings, including the generators for its invariant ring. This paper is organized as follows: Section 2 describes some properties of the ring  $B_k$  such as maximal ideals and automorphisms. Meanwhile, in Section 3, we describe a Gray map for the ring  $B_k$ , and we characterize linear codes and equivalent codes over the ring  $B_k$ . Finally, in Section 4, we characterize Euclidean self-dual codes, give the shape of MacWilliams relation and generators of invariant rings for Euclidean self-dual codes.

## 2. The ring $B_k$

As we readily see, the ring  $B_k$  forms a commutative algebra over prime field  $\mathbb{F}_p$ . Let  $\Omega = \{1, 2, \dots, k\}$  and  $2^\Omega$  is the collection of all subsets of  $\Omega$ . Also, let  $w_i$  be an element in the set  $\{v_i, 1 - v_i\}$ , for  $1 \leq i \leq k$ . Then, we will prove the following observation.

**Lemma 2.1.**  $\omega \in B_k$  is a zero divisor if and only if  $\omega \in \langle w_1, w_2, \dots, w_k \rangle$ .

**Proof.** ( $\Leftarrow$ ) It is clear that,  $v_i(1 - v_i) = 0$ , for all  $i = 1, \dots, k$ . Therefore, if  $\omega \in \langle w_1, w_2, \dots, w_k \rangle$ , then it is a zero divisor in  $B_k$ .

( $\Rightarrow$ ) Consider the equation,

$$(\alpha + \beta v_k)(\gamma + \epsilon v_k) = a + bv_k$$

given  $\alpha + \beta v_k, a + bv_k \in B_k$ , for some  $\alpha, \beta, a, b \in B_{k-1}$ . We have  $\gamma = a\alpha^{-1}$  and  $\epsilon = (b - \beta a)(\alpha(\beta + \alpha))^{-1}$ . Therefore, if  $a + bv_k = 1$ , then  $\gamma = 1$  and  $\epsilon = -\beta(\alpha(\beta + \alpha))^{-1}$ . Which implies,  $\alpha + \beta v_k$  is a unit if and only if  $\alpha$  and  $\alpha + \beta$  are also units. Considering this observation for elements in  $B_{k-1}, B_{k-2}, \dots, B_1$ , we have  $\alpha + \beta v \in B_1$  is a unit if and only if  $\alpha, \alpha + \beta \in \mathbb{F}_p$  are non zero elements. Since, every element in finite commutative ring is either a unit or a zero divisor, we can see that the only zero divisors in  $B_1$  are the elements in the ideals generated by  $\beta v$  or  $\alpha(1 - v)$ . By generalizing this result recursively, we have the intended conclusion.  $\square$

Also, we can easily show that  $I = \langle w_1, w_2, \dots, w_k \rangle$  is a maximal ideal in  $B_k$ .

**Lemma 2.2.** Let  $I = \langle w_1, w_2, \dots, w_k \rangle$ . Then  $I$  is a maximal ideal in  $B_k$ .

**Proof.** Consider quotient ring  $B_k/I$ . If  $v_i \in I$ , then  $1 - v_i \equiv 1 \pmod I$ , and if  $1 - v_i \in I$ , then  $v_i = 1 - (1 - v_i) \equiv 1 \pmod I$ . Consequently,  $B_k/I$  is a field. So,  $I$  is a maximal ideal. Moreover,  $B_k/I \cong \mathbb{F}_p$ .  $\square$

The following lemma is needed to prove Proposition 2.4.

**Lemma 2.3.**  $\alpha^p = \alpha$ , for all  $\alpha \in B_k$ .

**Proof.** Let  $\alpha = \sum_{A \subseteq \{1, \dots, k\}} \alpha_A v_A$ , for some  $\alpha_A \in \mathbb{F}_p$ , where  $v_A = \prod_{j \in A} v_j$ . Then, consider

$$\alpha^p = \sum_{i=0}^p \binom{p}{i} \alpha_{A_1}^i v_{A_1} \left( \sum_{A \neq A_1} \alpha_A v_A \right)^{p-i} = \alpha_{A_1} v_{A_1} + \left( \sum_{A \neq A_1} \alpha_A v_A \right)^p$$

since  $\mathbb{F}_p$  has characteristic  $p$  and  $\beta^{p-1} = 1$  for all  $\beta \in \mathbb{F}_p$ . If we continue this procedure, then we have  $\alpha^p = \alpha$ .  $\square$

The following result shows that the ring  $B_k$  is a principal ideal ring.

**Proposition 2.4.** Let  $I = \langle \alpha_1, \dots, \alpha_m \rangle$  be an ideal in  $B_k$ , for some  $\alpha_1, \dots, \alpha_m \in B_k$ . Then,

$$I = \left\langle \sum_{A \subseteq \{1, \dots, m\}, A \neq \emptyset} (-1)^{|A|+1} \left( \prod_{j \in A} \alpha_j \right)^{p-1} \right\rangle.$$

**Proof.** Consider  $\alpha_i \sum_{A \subseteq \{1, \dots, m\}, A \neq \emptyset} (-1)^{|A|+1} \left( \prod_{j \in A} \alpha_j \right)^{p-1}$ . For any  $A \subseteq \{1, \dots, m\}$ , if  $i \in A$ , then

$$\alpha_i (-1)^{|A|+1} \left( \prod_{j \in A} \alpha_j \right)^{p-1} = (-1)^{|A|+1} \alpha_i \left( \prod_{j \in A - \{i\}} \alpha_j \right)^{p-1}$$

since  $\alpha_i^p = \alpha_i$  by Lemma 2.3. Consequently, there is a unique  $A' = A - \{i\} \subseteq \{1, \dots, m\}$ , such that

$$\alpha_i \left( (-1)^{|A|+1} \left( \prod_{j \in A} \alpha_j \right)^{p-1} + (-1)^{|A'|+1} \left( \prod_{j \in A'} \alpha_j \right)^{p-1} \right) = 0.$$

Otherwise, if  $i \notin A$ , then there is a unique  $A'' = A \cup \{i\} \subseteq \{1, \dots, m\}$  such that

$$\alpha_i \left( (-1)^{|A|+1} \left( \prod_{j \in A} \alpha_j \right)^{p-1} + (-1)^{|A''|+1} \left( \prod_{j \in A''} \alpha_j \right)^{p-1} \right) = 0.$$

So, every term will be vanish except  $\alpha_i \alpha_i^{p-1} = \alpha_i$ . Therefore,

$$I \subseteq \left\langle \sum_{A \subseteq \{1, \dots, m\}, A \neq \emptyset} (-1)^{|A|+1} \left( \prod_{j \in A} \alpha_j \right)^{p-1} \right\rangle.$$

It is clear that

$$\left\langle \sum_{A \subseteq \{1, \dots, m\}, A \neq \emptyset} (-1)^{|A|+1} \left( \prod_{j \in A} \alpha_j \right)^{p-1} \right\rangle \subseteq I.$$

Thus,  $I = \left\langle \sum_{A \subseteq \{1, \dots, m\}, A \neq \emptyset} (-1)^{|A|+1} \left( \prod_{j \in A} \alpha_j \right)^{p-1} \right\rangle$ .  $\square$

The following proposition shows that the ideal in Lemma 2.2 is the only maximal ideal in  $B_k$ .

**Proposition 2.5.** An ideal  $I$  in  $B_k$  is maximal if and only if  $I = \langle w_1, w_2, \dots, w_k \rangle$ .

**Proof.** ( $\Leftarrow$ ) It is clear by Lemma 2.2.

( $\Rightarrow$ ) Let  $J$  be a maximal ideal in  $B_k$ . By Proposition 2.4,  $B_k$  is a principal ideal ring. Then, let  $J = \langle \omega \rangle$ , for some  $\omega \in B_k$ . Note that,  $\omega$  is not a unit in  $B_k$ , so it is a zero divisor. By Lemma 2.1,  $\omega$  is an element of some  $m_i = \langle w_1, w_2, \dots, w_k \rangle$ , which means  $J \subseteq m_i$ . Consequently,  $J = m_i$ , because  $J$  is a maximal ideal.  $\square$

Using the above result, we have the following lemmas.

**Lemma 2.6.** *The ring  $B_k$  can be viewed as an  $\mathbb{F}_p$ -vector space with dimension  $2^k$  whose basis consists of elements of the form  $w_S = \prod_{i \in S} w_i$ , where  $S \in 2^\Omega$ .*

**Proof.** As we can see, every element  $a \in B_k$  can be written as  $a = \sum_{S \in 2^\Omega} \alpha_S v_S$ , for some  $\alpha_S \in \mathbb{F}_p$ , where  $v_S = \prod_{i \in S} v_i$  and  $v_\emptyset = 1$ . So,  $B_k$  is a vector space over  $\mathbb{F}_p$  whose basis consists of elements of the form  $v_S = \prod_{i \in S} v_i$ , where  $v_\emptyset = 1$  and there are  $\sum_{j=0}^k \binom{k}{j} = 2^k$  elements of basis. Now, we will show that the set  $\{1, w_{S_2}, \dots, w_{S_{2^k}}\}$  is also a basis. Consider,

$$\alpha_1 + \alpha_2 w_{S_2} + \dots + \alpha_{2^k} w_{S_{2^k}} = 0$$

for some  $\alpha_i \in \mathbb{F}_p$ , for all  $i = 1, \dots, 2^k$ , which gives,

$$-\alpha_1 = \alpha_2 w_{S_2} + \dots + \alpha_{2^k} w_{S_{2^k}}.$$

If  $\alpha_1 \neq 0$ , then  $\xi_1 = (\alpha_2 w_{S_2} + \dots + \alpha_{2^k} w_{S_{2^k}})$  is a unit, a contradiction to the fact that  $\xi_1 \in \langle w_1, \dots, w_k \rangle$ . So,  $\alpha_1 = 0$ , which means,

$$-(\alpha_2 w_{S_2} + \dots + \alpha_{k+1} w_{S_{k+1}}) = \alpha_{k+2} w_{S_{k+2}} + \dots + \alpha_{2^k} w_{S_{2^k}}.$$

If  $(\alpha_2 w_{S_2} + \dots + \alpha_{k+1} w_{S_{k+1}}) \neq 0$ , then it is a contradiction to the fact that  $|S_j| \geq 2$ , for all  $j = k+2, \dots, 2^k$ . Consequently,  $(\alpha_2 w_{S_2} + \dots + \alpha_{k+1} w_{S_{k+1}}) = 0$ . We have to note that, the set with elements of the  $w_S$ , where  $S \in 2^\Omega$ , is also linearly independent over  $\mathbb{F}_p$ , because  $S_k$  is a vector space over  $\mathbb{F}_p$  with element of basis are of the form  $v_S$ , where  $S \subseteq \Omega$ . Therefore,  $(\alpha_2 w_{S_2} + \dots + \alpha_{k+1} w_{S_{k+1}}) = 0$  gives  $\alpha_2 = \dots = \alpha_{k+1} = 0$ . By continuing this process, we have  $\alpha_1 = \dots = \alpha_{2^k} = 0$ , which means they are linearly independent over  $\mathbb{F}_p$ .  $\square$

**Lemma 2.7.** *The ring  $B_k$  has characteristic  $p$  and cardinality  $p^{2^k}$ .*

**Proof.** It is immediate since characteristic of  $\mathbb{F}_p$  is  $p$ , and  $B_k$  can be viewed as a  $\mathbb{F}_p$ -vector space with dimension  $\sum_{i=0}^k \binom{k}{i} = 2^k$ . So,  $|B_k| = p^{2^k}$ .  $\square$

The following theorem characterizes the shape of automorphisms in the ring  $B_k$ .

**Theorem 2.8.** *Let  $\theta$  be an endomorphism in  $B_k$ . Then,  $\theta$  is an automorphism if and only if  $\theta(v_i) = w_j$ , for every  $i \in \Omega$ , and  $\theta$ , when restricted to  $\mathbb{F}_p$ , is an identity map.*

**Proof.** ( $\implies$ ) Let  $J = \langle v_1, \dots, v_k \rangle$  and  $J_\theta = \langle \theta(v_1), \dots, \theta(v_k) \rangle$ . Consider the map

$$\lambda: \frac{B_k}{J} \rightarrow \frac{B_k}{J_\theta} \\ a + J \mapsto \theta(a) + J_\theta$$

We can see that the map  $\lambda$  is a ring homomorphism. For any  $a, b \in B_k/J$  where  $\lambda(a) = \lambda(b)$ , let  $a = a_1 + J$  and  $b = b_1 + J$  for some  $a_1, b_1 \in B_k$ . As we can see,  $\theta(a_1 - b_1) \in J_\theta$ , so  $a_1 - b_1 \in J$ . Consequently,  $a - b = 0 + J$ , which means  $a = b$ , in other words,  $\lambda$  is a monomorphism. Moreover, for any  $a' \in B_k/J_\theta$ , let  $a' = a_2 + J_\theta$  for some  $a_2 \in B_k$ , then there exists  $a = \theta^{-1}(a_2) + J$  such that  $\lambda(a) = a'$ . Therefore,  $\mathbb{F}_p \simeq B_k/J \simeq B_k/J_\theta$ , which implies  $J_\theta$  is also a maximal ideal. By Proposition 2.5,  $J_\theta = \langle w_1, \dots, w_k \rangle$ , where  $w_i \in \{v_i, 1 - v_i\}$  for  $1 \leq i \leq k$ . By Proposition 2.4,

$$J_\theta = \langle \sum_{A \subseteq \Omega, A \neq \emptyset} (-1)^{|A|+1} (\prod_{j \in A} w_j)^{p-1} \rangle = \langle \sum_{A \subseteq \Omega, A \neq \emptyset} (-1)^{|A|+1} (\prod_{j \in A} \theta(v_j))^{p-1} \rangle$$

which means,  $\sum_{A \subseteq \Omega, A \neq \emptyset} (-1)^{|A|+1} (\prod_{j \in A} w_j)^{p-1}$  and  $\sum_{A \subseteq \Omega, A \neq \emptyset} (-1)^{|A|+1} (\prod_{j \in A} \theta(v_j))^{p-1}$  are associate. Therefore,  $\theta(v_i) = \beta w_j$  for some unit  $\beta$  which satisfies  $(\beta^{|A|})^{p-1} = \beta$ , for all  $A \neq \emptyset$ . Consequently, we

have  $\beta^{p-1} = \beta$ , but by Lemma 2.3,  $\beta^p = \beta$ . Since  $\beta$  is a unit, we have that  $\beta^{p-1} = 1$ . Therefore,  $\beta$  must be equal to 1. Moreover, since  $\theta$  is an automorphism,  $\theta(v_i) \neq \theta(v_j)$  whenever  $i \neq j$ . Also, since the only automorphism in  $\mathbb{F}_p$  is identity map, we have the conclusion.

( $\Leftarrow$ ) Suppose that  $\theta(v_i) = w_j$ , and  $\theta(v_i) \neq \theta(v_j)$  whenever  $i \neq j$ . By Lemma 2.6, we can see that  $\theta$  is also an automorphism.  $\square$

Now, we have to note that every element  $a$  in  $B_k$  can be written as

$$a = \sum_{S \in 2^\Omega} \alpha_S w_S$$

for some  $\alpha_S \in \mathbb{F}_p$ , where  $w_S = \prod_{i \in S} w_i$ . Define a map  $\varphi$  as follows.

$$\begin{aligned} \varphi : B_k &\rightarrow \mathbb{F}_p^{2^k} \\ a = \sum_{i=1}^{2^k} \alpha_{S_i} w_{S_i} &\mapsto (\sum_{S \subseteq S_1} \alpha_S, \sum_{S \subseteq S_2} \alpha_S, \dots, \sum_{S \subseteq S_{2^k}} \alpha_S) \end{aligned}$$

We can show that this map  $\varphi$  is a bijection map. Furthermore, this map can be extended  $n$  tuples of  $B_k$  as follows.

$$\begin{aligned} \bar{\varphi} : B_k^n &\rightarrow \mathbb{F}_p^{n2^k} \\ (a_1, \dots, a_n) &\mapsto (\varphi(a_1), \dots, \varphi(a_n)). \end{aligned}$$

Since  $\varphi$  is a bijection map, we also have  $\bar{\varphi}$  is a bijection map. We have to note that, the map  $\varphi$  is a permutation, based on the choice of subsets  $S_i \in 2^\Omega$ , of Gray maps in [2].

### 3. Codes over the ring $B_k$

A subset  $C \subseteq B_k^n$  is called *code* over  $B_k$  of length  $n$ . If  $C$  is a  $B_k$ -submodule of  $B_k^n$ , then  $C$  called *linear code*. The following proposition gives a characterization of  $B_k$ -linear codes using the map  $\bar{\varphi}$ .

**Proposition 3.1.**  *$C$  is a linear code over  $B_k$  if and only if there exist linear codes  $C_1, \dots, C_{2^k}$  over  $\mathbb{F}_p$  such that  $C = \bar{\varphi}^{-1}(C_1, \dots, C_{2^k})$ .*

**Proof.** ( $\Rightarrow$ ) Since  $\bar{\varphi}$  is a bijection, there exist  $C_1, \dots, C_{2^k}$  such that  $C = \bar{\varphi}^{-1}(C_1, \dots, C_{2^k})$ . Now, we only need to show that  $C_i$  is a linear code over  $\mathbb{F}_p$  for all  $i = 1, \dots, 2^k$ . For any  $C_i$ , let  $c_1$  and  $c_2$  be two codewords in  $C_i$ . For  $l = 1, 2$ , let  $c_l = (\alpha_1^{(l)}, \dots, \alpha_n^{(l)})$ , for some  $\alpha_j^{(l)}$  in  $\mathbb{F}_p$ . Consider

$$\begin{aligned} c'_l &= \bar{\varphi}^{-1}(\mathbf{0}, \dots, \mathbf{0}, \lambda_l c_l, \mathbf{0}, \mathbf{0}) \\ &= \left( \varphi^{-1}(0, \dots, 0, \lambda_l \alpha_1^{(l)}, 0, \dots, 0), \dots, \varphi^{-1}(0, \dots, 0, \lambda_l \alpha_n^{(l)}, 0, \dots, 0) \right) \\ &= \left( \lambda_l \alpha_1^{(l)} \left( w_{S_l} - \sum_{j \in \{1, \dots, k\} - S_l} w_{S_l \cup \{j\}} \right), \dots, \lambda_l \alpha_n^{(l)} \left( w_{S_l} - \sum_{j \in \{1, \dots, k\} - S_l} w_{S_l \cup \{j\}} \right) \right), \end{aligned}$$

for any  $\lambda_l$  in  $\mathbb{F}_p^\times$  for all  $l = 1, 2$ . The last equality holds since

$$\varphi \left( \alpha_t^{(l)} \left( w_{S_l} - \sum_{j \in \{1, \dots, k\} - S_l} w_{S_l \cup \{j\}} \right) \right) = (0, \dots, 0, \alpha_t^{(l)}, 0, \dots, 0)$$

for all  $1 \leq t \leq n$ . Since  $C = \bar{\varphi}^{-1}(C_1, \dots, C_{2^k})$ , we have  $c'_l$  is in  $C$  for all  $l = 1, 2$ , and  $c'_1 + c'_2$  is also in  $C$ . Then, consider

$$\overline{\varphi}(c'_1 + c'_2) = \begin{pmatrix} 0 & \cdots & 0 & \cdots & 0 \\ \vdots & \cdots & \vdots & \cdots & \vdots \\ 0 & \cdots & 0 & \cdots & 0 \\ \lambda_1 \alpha_1^{(1)} + \lambda_2 \alpha_1^{(2)} & \cdots & \lambda_1 \alpha_l^{(1)} + \lambda_2 \alpha_l^{(2)} & \cdots & \lambda_1 \alpha_n^{(1)} + \lambda_2 \alpha_n^{(2)} \\ 0 & \cdots & 0 & \cdots & 0 \\ \vdots & \cdots & \vdots & \cdots & \vdots \\ 0 & \cdots & 0 & \cdots & 0 \end{pmatrix}.$$

Hence,  $\lambda_1 c_1 + \lambda_2 c_2$  is also in  $C_i$ .

( $\Leftarrow$ ) Take any two codewords  $c_3$  and  $c_4$  in  $C$ . Let

$$c_3 = \left( \sum_{S \in 2^\Omega} \alpha_S^{(1)} w_S, \dots, \sum_{S \in 2^\Omega} \alpha_S^{(n)} w_S \right)$$

and

$$c_4 = \left( \sum_{S \in 2^\Omega} \beta_S^{(1)} w_S, \dots, \sum_{S \in 2^\Omega} \beta_S^{(n)} w_S \right),$$

for some  $\alpha_i, \beta_i$  in  $\mathbb{F}_p$ , where  $i = 1, \dots, 2^k$ . For any  $\lambda_3$  and  $\lambda_4$  in  $\mathbb{F}_p^\times$  we have

$$\overline{\varphi}(\lambda_3 c_3 + \lambda_4 c_4) = \begin{pmatrix} \lambda_3 \alpha_{S_1}^{(1)} + \lambda_4 \beta_{S_1}^{(1)} & \cdots & \lambda_3 \alpha_{S_1}^{(n)} + \lambda_4 \beta_{S_1}^{(n)} \\ \lambda_3 \sum_{S \subseteq S_2} \alpha_S^{(1)} + \lambda_4 \sum_{S \subseteq S_2} \beta_S^{(1)} & \cdots & \lambda_3 \sum_{S \subseteq S_2} \alpha_S^{(n)} + \lambda_4 \sum_{S \subseteq S_2} \beta_S^{(n)} \\ \vdots & \vdots & \vdots \\ \lambda_3 \sum_{S \subseteq S_{2^k}} \alpha_S^{(1)} + \lambda_4 \sum_{S \subseteq S_{2^k}} \beta_S^{(1)} & \cdots & \lambda_3 \sum_{S \subseteq S_{2^k}} \alpha_S^{(n)} + \lambda_4 \sum_{S \subseteq S_{2^k}} \beta_S^{(n)} \end{pmatrix}$$

is also in  $(C_1, \dots, C_{2^k})$ , since  $C_i$  is a linear code for every  $i = 1, \dots, 2^k$ . Therefore,  $\lambda_3 c_3 + \lambda_4 c_4$  is also in  $C$ .  $\square$

Now, following [5], we define permutation equivalence of codes as follows.

**Definition 3.2.** Two codes are permutation equivalent if one can be obtained from the other by permuting the coordinates.

Using Definition 3.2, we can define the following notion of equivalence between two codes.

**Definition 3.3.** Two codes  $C$  and  $C'$  over  $B_k$  are equivalent if either they are permutation-equivalent or  $C$  is permutation equivalent to the code  $\theta(C')$  for some automorphism  $\theta$  in  $B_k$ , i.e. the code  $\theta(C')$  obtained from  $C'$  by changing  $\alpha$  with  $\theta(\alpha)$  in all coordinates.

Note that, the above definition is similar to the one in [5]. Now, let  $\Pi_\theta$  be a permutation on  $2^k$  tuples of  $\mathbb{F}_p$  induced by automorphism  $\theta$ . Then we have

$$(\Pi_\theta \circ \overline{\varphi})(c) = \overline{\varphi}(\theta(c)) \quad (1)$$

for any  $c \in B_k^n$ . Then, we have the following characterization.

**Theorem 3.4.** Let  $C$  and  $C'$  be two codes over  $B_k$ . Then,  $C$  and  $C'$  are equivalent if and only if there exists a permutation which sends  $(C_1, \dots, C_{2^k})$  to  $(C'_1, \dots, C'_{2^k})$  or to  $(\Pi_\theta(C'_1), \dots, \Pi_\theta(C'_{2^k}))$ .

**Proof.** ( $\Rightarrow$ ) Let  $C = \bar{\varphi}^{-1}(C_1, \dots, C_{2^k})$  and  $C' = \bar{\varphi}^{-1}(C'_1, \dots, C'_{2^k})$ , where  $C_i$  and  $C'_i$  are codes over  $\mathbb{F}_p$ , for all  $1 \leq i \leq 2^k$ . If there exists an automorphism  $\theta$  such that  $C$  is permutation equivalent to  $\theta(C')$ , then by equation 1, we have  $C = \bar{\varphi}^{-1}(C_1, \dots, C_{2^k})$  is permutation equivalent to  $(\Pi_\theta(C'_1), \dots, \Pi_\theta(C'_{2^k}))$ .

( $\Leftarrow$ ) If there exists a permutation which sends  $(C_1, \dots, C_{2^k})$  to

$$(\Pi_\theta(C'_1), \dots, \Pi_\theta(C'_{2^k})),$$

for some bijective map  $\Pi_\theta$ , then we can have the automorphism  $\theta$  using the equation 1.  $\square$

## 4. Invariant ring

In this section, we describe some aspect of Euclidean self-dual codes as well as MacWilliams identity and invariant ring.

Related to Euclidean self-dual codes over the ring  $B_k$ , we have the following result.

**Proposition 4.1.** *Let  $C = \bar{\varphi}^{-1}(C_1, C_2, \dots, C_{2^k})$ , for some  $p$ -ary codes  $C_1, \dots, C_{2^k}$ . Then,  $C$  is Euclidean self-dual codes over  $B_k$  if and only if  $C_i$  is also Euclidean self-dual codes, for  $1 \leq i \leq 2^k$ .*

**Proof.** ( $\Rightarrow$ ) For any  $c_i \in C_i$ , let  $c_i = (\alpha_{S_i}^{(0)}, \dots, \alpha_{S_i}^{(n-1)})$ , for some  $\alpha_{S_i}^{(j)} \in \mathbb{F}_p$ , where  $0 \leq j \leq n-1$ . Let  $c = \bar{\varphi}^{-1}(0, \dots, 0, c_i, 0, \dots, 0) \in C$ , then we have  $\langle c, c' \rangle = 0$  for every  $c' \in C$ . To make the representation for any element in the ring  $B_k$  easier, we will use the basis whose elements are of the form  $v_S$ , for all  $S \subseteq \{1, 2, \dots, k\}$ . Now, let

$$c' = \left( \beta_{S_i}^{(0)} v_{S_i} + \sum_{S \in 2^\Omega, S \neq S_i} \beta_S^{(0)} v_S, \dots, \beta_{S_i}^{(n-1)} v_{S_i} + \sum_{S \in 2^\Omega, S \neq S_i} \beta_S^{(n-1)} v_S \right).$$

Consider,

$$\begin{aligned} c &= \bar{\varphi}^{-1}(0, \dots, 0, c_i, 0, \dots, 0) \\ &= \left( \alpha_{S_i}^{(0)} (v_{S_i} - \sum_{j \in \{1, \dots, k\} - S_i} v_{S_i \cup \{j\}}), \dots, \alpha_{S_i}^{(n-1)} (v_{S_i} - \sum_{j \in \{1, \dots, k\} - S_i} v_{S_i \cup \{j\}}) \right). \end{aligned}$$

Since  $\langle c, c' \rangle = 0$  for every  $c' \in C$  and  $v_S^2 = v_S$  for every  $S \in 2^\Omega$ , we have

$$\sum_{j=0}^{n-1} \left( \alpha_{S_i}^{(j)} \beta_{S_i}^{(j)} v_{S_i} - \sum_{j \in \{1, \dots, k\} - S_i} \alpha_{S_i}^{(j)} \beta_{S_i \cup \{j\}}^{(j)} v_{S_i \cup \{j\}} = 0 \right).$$

Consequently,  $\sum_{j=0}^{n-1} \alpha_{S_i}^{(j)} \beta_{S_i}^{(j)} = 0$ .

Take any  $c'_i \in C_i$ . Let  $c'_i = (\gamma_{S_i}^{(0)}, \dots, \gamma_{S_i}^{(n-1)})$ , for some  $\gamma_{S_i}^{(j)} \in \mathbb{F}_p$ , where  $0 \leq j \leq n-1$ . Since  $c' = \bar{\varphi}^{-1}(0, \dots, 0, c'_i, 0, \dots, 0) \in C$ , we have  $\langle c, c' \rangle = 0$ . So

$$\langle c_i, c'_i \rangle = \sum_{j=0}^{n-1} \alpha_{S_i}^{(j)} \gamma_{S_i}^{(j)} = 0.$$

Therefore  $C_i \subseteq C_i^\perp$ .

For any  $c_1 \in C_1$ , let  $c_1 = (\zeta_0, \dots, \zeta_{n-1})$  for some  $\zeta_j \in \mathbb{F}_p$ , where  $0 \leq j \leq n-1$ . Since  $\langle c_1, c_i \rangle = 0$ , we have  $\sum_{j=0}^{n-1} \zeta_j \alpha_{S_i}^{(j)} = 0$ . We can see that

$$\begin{aligned} c'_1 &= \bar{\varphi}^{-1}(0, \dots, 0, c_1, 0, \dots, 0) \\ &= \left( \zeta_0 (v_{S_i} - \sum_{j \in \{1, \dots, k\} - S_i} v_{S_i \cup \{j\}}), \dots, \zeta_{n-1} (v_{S_i} - \sum_{j \in \{1, \dots, k\} - S_i} v_{S_i \cup \{j\}}) \right). \end{aligned}$$

Now, since  $\sum_{j=0}^{n-1} \zeta_j \alpha_{S_i}^{(j)} = 0$ , we also have  $\langle c'_1, c_2 \rangle = 0$  for every  $c_2 \in C$ . Remember that  $C = C^\perp$ , which gives  $c'_1 \in C$ . So,  $c_1 \in C_i$ , or in other words  $C_i^\perp \subseteq C_i$ . Thus,  $C_i$  is a Euclidean self-dual code, for all  $i = 1, \dots, 2^k$ .

( $\Leftarrow$ ) Take any  $c_1, c_2 \in C$ . For every  $i = 1, 2$ , let

$$c_i = \left( \sum_{S \subseteq \{1, \dots, k\}} c_S^{(i,0)}, \dots, \sum_{S \subseteq \{1, \dots, k\}} c_S^{(i,n-1)} \right),$$

for some  $c_S^{(i,j)} \in \mathbb{F}_p$ , where  $i = 1, 2$ , and  $j = 0, \dots, n-1$ . Consider,

$$\begin{aligned} \bar{\varphi}(c_i) = & \left( \sum_{S \subseteq S_1} c_S^{(i,0)}, \dots, \sum_{S \subseteq S_1} c_S^{(i,n-1)}, \dots \right. \\ & \dots, \sum_{S \subseteq S_l} c_S^{(i,0)}, \dots, \sum_{S \subseteq S_l} c_S^{(i,n-1)}, \dots \\ & \left. \dots, \sum_{S \subseteq S_{2^k}} c_S^{(i,0)}, \dots, \sum_{S \subseteq S_{2^k}} c_S^{(i,n-1)} \right), \end{aligned}$$

where  $i = 1, 2$ . Since  $C_l$  is a Euclidean self-dual code, for all  $l = 1, \dots, 2^k$ , we have

$$\begin{aligned} \langle c_1, c_2 \rangle &= \sum_{j=0}^{n-1} \sum_{S_l \in 2^\Omega} \sum_{S \subseteq S_l} c_S^{(1,j)} c_S^{(2,j)} v_S \\ &= 0. \end{aligned}$$

So,  $C \subseteq C^\perp$ .

Now, take any  $c_3 \in C^\perp$ . Since  $\langle c_3, c \rangle = 0$  for all  $c \in C$ , we have

$$\sum_{j=0}^{n-1} \sum_{S \subseteq S_l} c_S^{(1,j)} c_S^{(2,j)} v_S = 0,$$

for all  $S \in 2^\Omega$ . Remember that  $C_l$  is a Euclidean self-dual code, for all  $l = 1, 2, \dots, 2^k$ , which give

$$\sum_{j=0}^{n-1} \sum_{S \subseteq S_l} c_S^{(1,j)} c_S^{(2,j)} v_S = 0,$$

for all  $S \in 2^\Omega$ , and moreover  $c_3 \in C$ . So,  $C^\perp \subseteq C$ . Therefore,  $C$  is a Euclidean self-dual code.  $\square$

The following lemma gives MacWilliams identity for codes over the ring  $B_k$ .

**Lemma 4.2.** *The MacWilliams identity for Hamming weight enumerators for codes over  $B_k$  is :*

$$W_{C^\perp}(X, Y) = \frac{1}{|C|} W_C(X + (p^{2^k} - 1)Y, X - Y) \quad (2)$$

**Proof.** The identity follows from [7, Theorem 8.3] and Proposition 4.1.  $\square$

As we can see from Lemma 4.2, MacWilliams identity gives a transformation between polynomial representing a code and polynomial representing its corresponding dual code. We have to note that if  $C$  is an Euclidean self-dual code, then the weight enumerator of  $C$  is invariant under this transformation. The above transformation can be formulated as an action 'o' by a matrix group  $G$  generated by matrices

$T = \begin{pmatrix} \frac{1}{p^{2^k-1}} & \frac{p^{2^k}-1}{p^{2^k-1}} \\ \frac{1}{p^{2^k-1}} & \frac{-1}{p^{2^k-1}} \end{pmatrix}$  and  $D = \begin{pmatrix} -1 & 0 \\ 0 & -1 \end{pmatrix}$ . The action of any  $g = \begin{pmatrix} a_1 & a_2 \\ a_3 & a_4 \end{pmatrix} \in G$  to a polynomial  $f(X, Y)$  is written as

$$g \circ f(X, Y) = f(a_1 X + a_2 Y, a_3 X + a_4 Y).$$

Note that the matrix  $T$  is derived from the identity in Lemma 4.2 and the matrix  $D$  is derived from the condition that  $n$  is always even. Also, it is easy to see that  $G = \{I, D, T, -T\}$ . Formally, we have the following result.

**Lemma 4.3.** *If  $W_C(X, Y)$  is a Hamming weight enumerator for an Euclidean self-dual code  $C$  over  $B_k$ , then  $W_C(X, Y)$  is invariant under the action of  $G$ .*

Let  $R_G$  be a set of all polynomials in two variables which are invariant under the action  $\circ$  of  $G$ . We can easily prove that  $R_G$  is a ring, and by the above Lemma we can see that every Hamming weight enumerator of Euclidean self-dual codes must be inside  $R_G$ . This ring  $R_G$  called *invariant ring* for Euclidean self-dual codes over  $B_k$ . The following theorem gives generators for  $R_G$ .

**Theorem 4.4.** *Invariant ring of  $G$  is generated by*

$$W_{C_0}(x, y) = x^2 + (p^{2^k} - 1)y^2$$

and

$$\tilde{f}(x, y) = \frac{1}{4} \left( \frac{2p^{2^{k-1}} + 2}{p^{2^k}} x^2 + \frac{4(p^{2^k} - 1)}{p^{2^{k-1}}} xy + \frac{2(p^{2^k} - 1)^2}{p^{2^{k-1}}} y^2 \right).$$

**Proof.** Consider the Molien series,

$$\begin{aligned} \Phi(\lambda) &= \frac{1}{|G|} \sum_{A \in G} \frac{1}{\det(I - \lambda A)} \\ &= \frac{1}{4} \left( \frac{1}{(1+\lambda)^2} + \frac{1}{(1-\lambda)^2} + \frac{2}{(1-\lambda^2)} \right) \\ &= \frac{1}{(1-\lambda^2)^2} \\ &= 1 + 2\lambda^2 + 3\lambda^4 + 4\lambda^6 + 5\lambda^8 + \dots + n\lambda^{2(n-1)} + \dots \end{aligned}$$

we can see that, the invariant ring generated by two invariants of degree 2. Consider the weight enumerator for self-dual code

$$C_0 = \{cc | \forall c \in A_k\}$$

i.e.  $W_{C_0}(x, y) = x^2 + (p^{2^k} - 1)y^2$ . This weight enumerator is of degree 2 and invariant under the action of  $G$ . So, this weight enumerator is one of the generator. We use averaging method to find the other one. Let  $f(x) = x^2$ , then by averaging method, we have

$$\tilde{f}(x, y) = \frac{1}{4} \left( \frac{2p^{2^{k-1}} + 2}{p^{2^k}} x^2 + \frac{4(p^{2^k} - 1)}{p^{2^{k-1}}} xy + \frac{2(p^{2^k} - 1)^2}{p^{2^{k-1}}} y^2 \right)$$

$\tilde{f}(x, y)$  are algebraically independent. □

## References

- [1] T. Abualrub, N. Aydin, P. Seneviratne, On  $\theta$ -cyclic codes over  $\mathbb{F}_2 + v\mathbb{F}_2$ , Australas. J. Combin. 54 (2012) 115–126.
- [2] Y. Cengellenmis, A. Dertli, S. T. Dougherty, Codes over an infinite family of rings with a Gray map, Des. Codes Cryptogr. 72(3) (2014) 559–580.
- [3] J. Gao, Skew cyclic codes over  $\mathbb{F}_p + v\mathbb{F}_p$ , J. Appl. Math. Inform. 31(3–4) (2013) 337–342.

- [4] A.R. Hammons, P. V. Kumar, A. R. Calderbank, N. J. A. Sloane, P. Sole, The  $\mathbb{Z}_4$ -linearity of Kerdock, Preparata, Goethals and related codes, *IEEE Trans. Inform. Theory* 40(2) (1994) 301–319.
- [5] W. Huffman, V. Pless, *Fundamentals of Error Correcting Codes*, Cambridge University Press, 2003.
- [6] Irwansyah, I. Muchtadi-Alamsyah, A. Muchlis, A. Barra, D. Suprijanto, Construction of  $\theta$ -cyclic codes over an algebra of order 4, *Proceeding of the Third International Conference on Computation for Science and Technology (ICCST-3)*, Atlantis Press, 2015.
- [7] J. Wood, Duality for modules over finite rings and applications to coding theory, *Amer. J. Math.* 121(3) (1999) 555–575.
